# Supplementary material for: Learning Beyond Rigid Manipulation with Hybrid Soft-Rigid Robots
Source: arXiv:2410.07787 source file (2026-11-09)
Supplement: Supplementary file 1 [file Supplementary.tex]

\documentclass[10pt]{article}
\usepackage{scicite}
\usepackage{color}
\usepackage{times}
\usepackage{mathtools}
\usepackage{amsmath}
\usepackage{amssymb}
\usepackage{bm}
\usepackage{url}
\usepackage[margin=1in]{geometry}

\begin{document}

\title{Supplementary Materials} \date{}
\maketitle 

\section*{Materials and Methods: Additional Technical Details}

\subsection*{Platform: Detailed technical description}

%
% Rigid
%
The proposed platform is a series interconnection of a rigid manipulator and a soft one. The main components of our hybrid platform are a rigid 7-DoF Franka Emika Panda robotic manipulator and a soft cable-driven arm. We utilize impedance control on the rigid manipulator, which enables us to easily provide kinesthetic demonstrations by making the robot compliant. 
For perception, we utilize a RealSense D405 depth camera. This is used for detecting keypoints and thus generalizing our skills to new situations. We use AprilTags for keypoint localization: each relevant object in the scene is marked with a tag, and the camera is used to retrieve their 3D positions in the robot's coordinate frame. These locations are then used to define the task-specific keypoints for both the demonstration and test-time scenarios. 

%During demonstrations, the user actuates the soft arm via buttons mounted on the Franka end-effector. Each button triggers a specific action on the two Dynamixel servos that tension the tendons within the soft structure—clockwise or counter-clockwise actuation, either individually or simultaneously. Tendon states and robot poses are logged in real time. During execution, the same motor commands are replayed from a microcontroller, following the reference trajectories predicted by the learned policy.

%\subsection*{Platform: Soft Cable-Driven Arm}

%
% Soft
%
The soft robotic arm is inspired by the movement and function of an octopus arm (see Figure \ref{SoftArm}). Its unique geometric design allows it to easily interact with objects of different shapes and sizes, making it well-suited for working in confined or complex environments. With a total length of 380 mm, it can conform to and securely grasp a wide range of objects, enabling robust yet adaptable manipulation. 
The arm follows a tapered morphology, with a base diameter of 35 mm that gradually decreases to 7 mm at the tip. This gradual transition enhances its ability to perform delicate and precise manipulations, closely mimicking the fine motor control observed in cephalopod appendages. Fabricated from Ecoflex 00-50, the structure exhibits exceptional flexibility and resilience. This material choice allows the arm to undergo large deformations, accommodating bending, twisting, and shape adaptation in response to external forces and environmental interactions (Figure \ref{SoftArm}A).

\begin{figure}[th]
\centering
\includegraphics[width=1\linewidth]{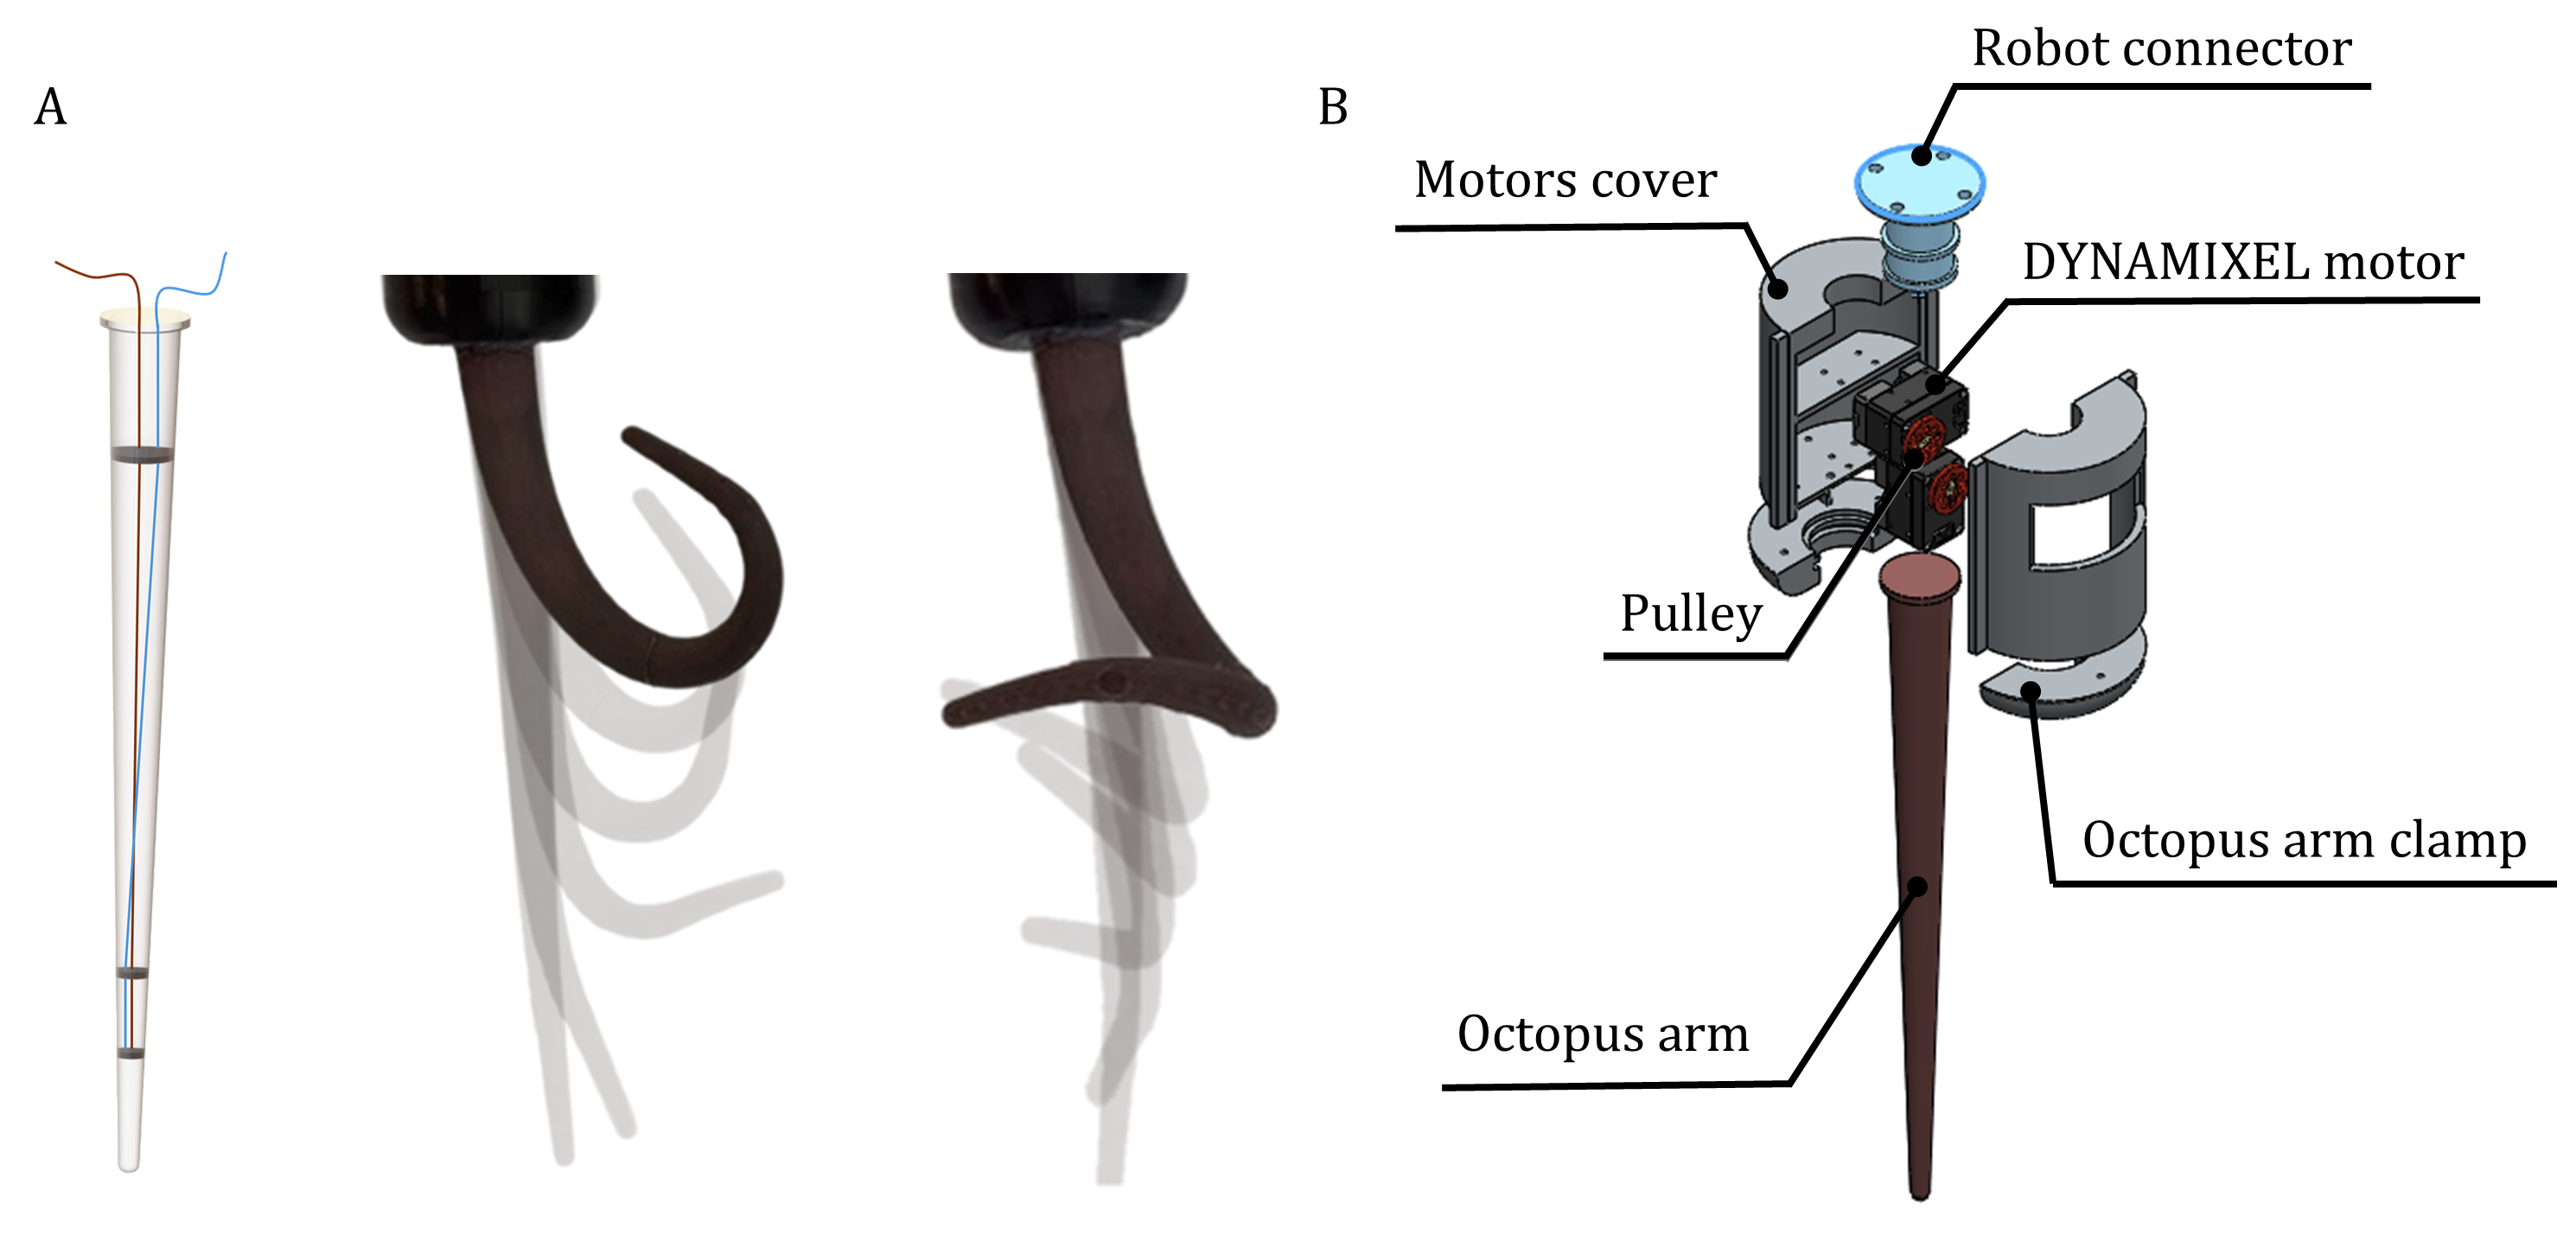}
\caption{\textbf{Design and actuation of the soft robotic arm.}  
(A) From left to right: the arm in its neutral state; executing a ventral bending motion via the blue cable; and performing a twisting motion via the magenta cable.  
The top row illustrates the internal routing of actuation cables, with blue controlling bending and magenta controlling twist.  
(B) Exploded view of the actuation module, showing two Dynamixel motors, a pulley system, and the octopus-inspired soft arm.  
The clamp secures the arm, while the robot connector enables attachment to the main manipulator.}
\label{SoftArm}
\end{figure}

Actuation is achieved through a cable-driven mechanism, where tensioned cables are routed through the arm and manipulated via pulleys actuated by a DYNAMIXEL MX-28 servo motor (Figure \ref{SoftArm}B). These are inside the black cylindrical casing, shown in Figure \ref{SoftArm}. More details on the low-level control loop implemented at the motor level are provided below. During execution, we can control the movement of the servos using an attached microcontroller.
This system enables independent control of two primary motion modes: twisting and bending. The twisting motion is actuated by a cable (marked in blue) that enters from the lower left side of the arm, reverses direction approximately one-quarter of the way along its length, and extends toward the upper right corner, allowing for controlled and continuous rotation. The bending motion is governed by a second cable (marked in brown), which runs along the arm's longitudinal axis. Upon actuation, this cable induces ventral bending, closely resembling the controlled flexion observed in biological octopus arms.

\subsection*{Design and Fabrication of Soft Robotic Tentacle}

The soft tentacle was fabricated through a multi-step process, as shown in Figure \ref{fig:FabricationProcess}. All components were designed in the SolidWorks software. The outer molds, which define the shape and external geometry of the tentacle, were fabricated using a Prusa 3D printer (i3 MK3S) with PLA filament. To ensure precision in the internal guideline parts —represented in black in the schematic—these were fabricated using a Formlabs Form 3 SLA printer with clear resin. The higher resolution and surface quality of SLA printing made it suitable for producing internal components that directly affect the performance and mechanical behavior of the final structure. Ecoflex 00-50 (Smooth-On Inc.), a silicone elastomer, was used as the structural material. Equal parts of Part A and Part B were measured and thoroughly mixed in a 1:1 weight ratio until a homogeneous mixture of materials was obtained. To remove air bubbles introduced during mixing, the silicone mixture was placed in a vacuum chamber and degassed until no further bubbles were observed.

Before casting, two flexible actuation cables—shown in blue and brown in the schematic—were inserted through the guiding channels within the mold. These cables were carefully positioned and fixed to a fixed alignment during the casting and curing process, as they are later used to drive the bending and twisting motions of the soft tentacle. Once the cables and internal parts were in place, the degassed silicone was poured into the assembled mold. The filled mold was then left to cure at room temperature. After curing, the mold was opened, and the soft tentacle was gently released, resulting in a fully formed soft tentacle with embedded internal features and integrated actuation cables.

\begin{figure}[th!]
    \centering
    \includegraphics[width=0.95\linewidth]{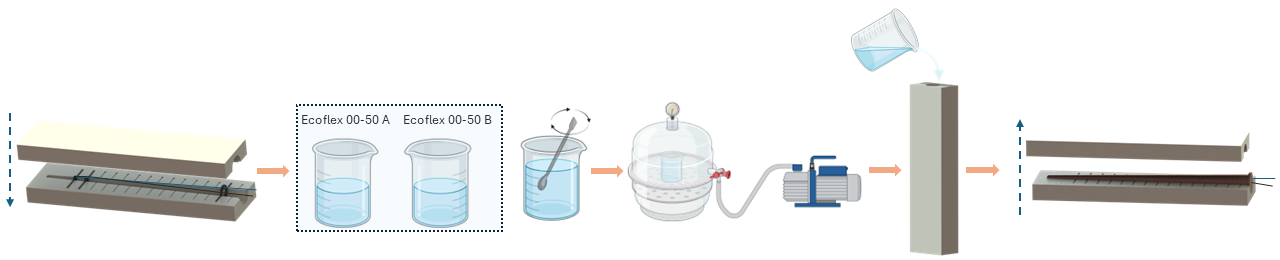}
    \caption{\textbf{Fabrication process of the soft tentacle.}  
    The process begins with mold assembly, followed by mixing equal parts of Ecoflex 00-50 A/B. The silicone mixture is degassed in a vacuum chamber to eliminate air bubbles, then cast into the mold with pre-positioned actuation cables. After curing at room temperature, the mold is opened to extract the final soft structure with embedded tendons.}
    %Fabrication process of the soft tentacle involves mold assembly, silicone mixing (Ecoflex 00-50 A/B), degassing, casting, and demolding.}
    \label{fig:FabricationProcess}
\end{figure}

\subsection*{Low-level Collocated Control loop and Its Stability}
To regulate the shape of the soft robot, we adopt a collocated PD control scheme in actuation coordinates, where each control loop regulates the length \( l_i \) of each of the two tendons via
\[
\tau_i = K_{\mathrm{P}} e_i+ K_{\mathrm{D}} \dot{e}_i, \quad e_i = l_i^{\mathrm{ref}} - l_i,
\]
where \( K_{\mathrm{P}}, K_{\mathrm{D}} \in \mathbb{R} \) are control gains, \( \tau_i \) is the torque applied to the motor driving the \(i\)-th tendon, and \( e_i \) is the tracking error between the reference and measured tendon length. 
Note that, without an integral term, this controller will not, in general, converge to zero regulation error. This, however, is not an issue in our context, as the reference to the controller is provided by the user during the demonstration, which generates the necessary reference to solve the task, regardless of the steady-state error. Instead, we are very interested in repeatability: the same reference evolution $l_i^{\mathrm{ref}}(t)$ should generate the same evolution in shape space. First, this motivates avoiding the use of an integrator, as it could modify the control output via its inner state. Second, we must ensure that the closed loop is globally exponentially convergent to the equilibrium. We will discuss this second point in more detail.

Let us denote by \( q = (q_{\mathrm{a}}, q_{\mathrm{u}}; q_{\mathrm{r}}) \) the full configuration vector of the robot, decomposed into actuated coordinates \( q_{\mathrm{a}} \) (tendon lengths), unactuated elastic coordinates \( q_{\mathrm{u}} \) (e.g., internal deformation modes), and rigid body coordinates \( q_{\mathrm{r}} \) (pose of the base manipulated by a rigid arm). The total potential energy is then defined as
\[
U(q_{\mathrm{a}}, q_{\mathrm{u}}; q_{\mathrm{r}}) = U_{\mathrm{elastic}}(q_{\mathrm{a}}, q_{\mathrm{u}}) + U_{\mathrm{gravity}}(q_{\mathrm{a}}, q_{\mathrm{u}}; q_{\mathrm{r}}).
\]
The elastic term is typically expressed as a quadratic function:
\[
U_{\mathrm{elastic}}(q_{\mathrm{a}}, q_{\mathrm{u}}) = \frac{1}{2} q_{\mathrm{u}}^\top K_{\mathrm{u}}(q_{\mathrm{a}}, q_{\mathrm{u}}) q_{\mathrm{u}},
\]
where \( K_{\mathrm{u}} \succ 0 \) is a configuration-dependent stiffness matrix arising from the nonlinear continuum mechanics of the structure. The gravitational potential is modeled as
\[
U_{\mathrm{gravity}}(q_{\mathrm{a}}, q_{\mathrm{u}}; q_{\mathrm{r}}) = - \int \rho(\alpha) \, g \, x_{\mathrm{g}}(\alpha; q_{\mathrm{a}}, q_{\mathrm{u}}; q_{\mathrm{r}}) \, d\alpha,
\]
where \( \alpha \) is the material abscissa along the body, \( x_{\mathrm{g}} \) denotes the projection of the spatial embedding along the gravity direction, and \( \rho(\alpha) \) is the local mass density. This term couples all configuration variables and contributes nontrivially to the total potential.

As a low-level controller for the rigid robot, we utilize the off-the-shelf controllers of the Franka Manipulator, which feature a PD control with gravity compensation. To prove the stability of the overall closed loop, we can employ 
\begin{equation}
    \begin{split}
        V & =  \frac{1}{2}
        \begin{bmatrix}
            \dot{q}_{\mathrm{r}}\\
            \dot{q}_{\mathrm{a}}\\
            \dot{q}_{\mathrm{u}}
        \end{bmatrix}^{\top}
        \begin{bmatrix}
            B_{\mathrm{r},\mathrm{r}}(q_{\mathrm{r}}, q_{\mathrm{a}}, q_{\mathrm{u}}) & B_{\mathrm{r},\mathrm{a}}(q_{\mathrm{r}}, q_{\mathrm{a}}, q_{\mathrm{u}}) & B_{\mathrm{r},\mathrm{u}}(q_{\mathrm{r}}, q_{\mathrm{a}}, q_{\mathrm{u}}) \\
            B_{\mathrm{r},\mathrm{a}}^{\top}(q_{\mathrm{r}}, q_{\mathrm{a}}, q_{\mathrm{u}}) & B_{\mathrm{a},\mathrm{a}}(q_{\mathrm{a}}, q_{\mathrm{u}}) & B_{\mathrm{a},\mathrm{u}}(q_{\mathrm{a}}, q_{\mathrm{u}}) \\
            B_{\mathrm{r},\mathrm{u}}^{\top}(q_{\mathrm{r}}, q_{\mathrm{a}}, q_{\mathrm{u}}) & B_{\mathrm{a},\mathrm{u}}^{\top}(q_{\mathrm{a}}, q_{\mathrm{u}}) & B_{\mathrm{u},\mathrm{u}}(q_{\mathrm{a}}, q_{\mathrm{u}})
        \end{bmatrix}
        \begin{bmatrix}
            \dot{q}_{\mathrm{r}}\\
            \dot{q}_{\mathrm{a}}\\
            \dot{q}_{\mathrm{u}}
        \end{bmatrix} 
        \\ & 
        + \left( U_{\mathrm{gravity}}(q_{\mathrm{a}}, q_{\mathrm{u}}; q_{\mathrm{r}}) - U_{\mathrm{gravity}}(q_{\mathrm{a}}^*, q_{\mathrm{u}}^*; q_{\mathrm{r}}^*) \right)
        + \left( U_{\mathrm{elastic}}(q_{\mathrm{a}}, q_{\mathrm{u}}) - U_{\mathrm{elastic}}(q_{\mathrm{a}}^*, q_{\mathrm{u}}^*) \right)
        \\ & 
        + \left( 
        \left. \nabla_{(q_{\mathrm{a}}, q_{\mathrm{u}})} \left( U_{\mathrm{elastic}} + U_{\mathrm{gravity}} \right) \right|_{(q_{\mathrm{a}}^*, q_{\mathrm{u}}^*; q_{\mathrm{r}}^*)}
        \right)^\top
        \begin{bmatrix}
            q_{\mathrm{a}}^* - q_{\mathrm{a}} \\
            q_{\mathrm{u}}^* - q_{\mathrm{u}}
        \end{bmatrix}
        \\ &
        + \frac{1}{2} (q^{*}_{\mathrm{r}} - q_{\mathrm{r}})^\top K_{P,r} (q^{*}_{\mathrm{r}} - q_{\mathrm{r}})
        + \frac{1}{2} (q^{*}_{\mathrm{a}} - q_{\mathrm{a}})^\top K_{P} (q^{*}_{\mathrm{a}} - q_{\mathrm{a}}).
    \end{split}
\end{equation}
where where \( B_{\mathrm{r},\mathrm{r}} \), \( B_{\mathrm{r},\mathrm{a}} \), \( B_{\mathrm{r},\mathrm{u}} \), \( B_{\mathrm{a},\mathrm{a}} \), \( B_{\mathrm{a},\mathrm{u}} \), and \( B_{\mathrm{u},\mathrm{u}} \) are the sub-blocks of the generalized inertia matrix associated with the rigid coordinates \( q_{\mathrm{r}} \), the actuation coordinates \( q_{\mathrm{a}} \), and the unactuated soft coordinates \( q_{\mathrm{u}} \), \( \nabla_{(q_{\mathrm{a}}, q_{\mathrm{u}})} \left( U_{\mathrm{elastic}} + U_{\mathrm{gravity}} \right) \) denotes the gradient of the total potential with respect to the internal and actuation coordinates, evaluated at the equilibrium configuration \( (q_{\mathrm{a}}^*, q_{\mathrm{u}}^*; q_{\mathrm{r}}^*) \) corresponding to the given reference inputs. The matrix \( K_{P,r} \) is the proportional gain of the rigid robot controller, which effectively acts as a virtual stiffness potential that penalizes deviations from the rigid base posture.

For $K_{P,r},K_{P}$ high enough, the only condition left for global asymptotic stability is that for any fixed \( (q_{\mathrm{a}}, q_{\mathrm{r}}) \), the total potential \( U(q_{\mathrm{a}}, \cdot ; q_{\mathrm{r}}) \) is strictly convex in \( q_{\mathrm{u}} \). This condition is usually referred to as (global) elastic dominance in soft robotics. This ensures that the internal dynamics possess a unique equilibrium configuration \( q_{\mathrm{u}}^*(q_{\mathrm{a}}, q_{\mathrm{r}}) \), globally attractive under damping or implicit mechanical dissipation. The system thus exhibits \emph{global elastic dominance}, a structural property that guarantees well-posedness and predictability of the shape response under tendon length control. In fabricating our soft arm (see above), we empirically sought a material that was soft enough to facilitate the desired level of physical intelligence during interactions, yet stiff enough to verify the elastic dominance conditions in all tested configurations.

\subsection*{Learning of the Process Transportation $\Phi$}

%\textbf{For Mariano}: {\color{red} Add here the details of the model used to learn the transformation map, and the training strategy. Start from Giovanni's paper, but modify the notation to make it coherent with the main text. Also, add more technical details on the actual implementation of the method.}
%
% Focus on the map learning part, copy initial part from here
%

%
Starting from a demonstration \((\tilde{{\mathcal{S}}}, {\mathcal{X}}, {\mathcal{R}}, {\mathcal{L}})\), where \(\tilde{\mathcal{S}}\) are the source task-level keypoints, \( \mathcal{X} \) the recorded cartesian positions, \( \mathcal{R} \) the orientations, and \( \mathcal{L} \) the servo configurations, our goal is to find a new sequence of robot states, \( \hat{\mathcal{{X}}}, \hat{\mathcal{{R}}}, \hat{\mathcal{{L}}} \) given the new target keypoints $\tilde{\mathcal{T}}$.
As described in the main text, we first map task-level keypoints to robot-centric keypoints.
For each source keypoint $\tilde{s_i}$ in $\tilde{\mathcal{S}}$, we find its closest point $s_i$ on the demonstrated Cartesian trajectory $\mathcal{X}$:
\begin{equation}
    {{s}}_i = \arg\min_{{x} \in {\mathcal{X}}} \lVert {x} - \tilde{s}_i \rVert.
\end{equation}
which results in the robot-centric set of keypoints $\mathcal{S}$.
In practice, for each source point $\tilde{s}_i$ we can shift the entire trajectory $X$ using $\tilde{s}_i$ to obtain a new trajectory $X_{s_{i}}$.
Then, by calculating the Euclidean norm of each point in $X_{s_{i}}$ and finding the point with the smallest norm, we can find our new robot-centric source point $s_i$.
Similarly, at execution time, we can now find the robot-centric target keypoints as ${t}_i = \tilde{t}_i + ({s}_i - \tilde{s}_i)$, resulting in the set $\mathcal{T}$.
Now we can learn a deformation map \({\Phi}_\mathcal{T}\) such that \({\mathcal{T}} = {\Phi}_\mathcal{T}({\mathcal{S}})\), and with this deformation map, find the new, generalized policy as:
\begin{equation}
    {\hat{\mathcal{X}}}(p) = {\Phi}_\mathcal{T}({\mathcal{X}}(p)), \quad 
    {\hat{\mathcal{R}}}(p) = {J}_\mathcal{T}({\mathcal{X}}(p)) {\mathcal{R}}(p), \quad 
    {\hat{\mathcal{L}}}(p) = {\mathcal{L}}(p),
    \label{eq:transporation}
\end{equation}
where $p$ is our progress (time) variable. To learn this map, as mentioned in the Method and Materials section, we separate the learning into a linear ($\gamma$) and a non-linear ($\psi$) part:
\begin{equation}
    \Phi_{\mathcal{T}} (x) = \gamma (x)+ \psi (\gamma (x)) .
\end{equation}
Note that the non-linear part $\psi (\gamma(x))$ is only fit on the residual error after applying the linear transformation $\gamma$(x).
To find the linear transformation $\psi$ we first find the centroids of the source and target distributions, $s_c$ and $t_c$.
We can then find the linear transformation $\gamma$ which best matches the centered source and target distributions:
\begin{equation}
    \mathcal{T} - t_c = \gamma (\mathcal{S} - s_c) .
\end{equation}
Through Singular Value Decomposition (SVD), we can first find the optimal rotation matrix $A$ between the two centered distributions if we impose
\begin{equation}
    U \Sigma V^\top = (\mathcal{S} - s_c)^\top (\mathcal{T} - t_c) ,
\end{equation}
where our desired rotation matrix $A$ will then be
\begin{equation}
    A = V U^\top .
\end{equation}
Thus, finally, we find the linear transformation as
\begin{equation}
    \gamma(x) = {A} (x - {s}_c) + {t}_c .
\end{equation}
Using the fitted linear part $\gamma$, we now want to find the non-linear part $\psi$ such that,
\begin{equation}
    \mathcal{T} - \gamma(\mathcal{S}) = \psi(\gamma(\mathcal{S}) ).
    \label{eq:psi_equality}
\end{equation}
This last non-linear part $\psi$ can in practice be learned with any regressor, such as an Multi-layer Perceptron or a Gaussian Process (GP).
We prefer to choose a GP due to its out-of-distribution properties: we can pick a zero-mean prior, which means that for points from the demonstration $\mathcal{X}$ which are \textit{far} away from the source keypoints $\mathcal{S}$, the total transformation ${\Phi}_{\mathcal{T}}$ will converge to only the linear part $\psi$.
This is desirable since, for our class of tasks, there will be points from the demonstrations that are far away from the keypoints, and we do not want to predict the non-linear deformation for these points where we lack information. 
Fitting a GP to act as our non-linear transformation $\psi$ in \eqref{eq:psi_equality} means we are training a GP with a dataset $ X = \gamma(\mathcal{S})$, and labels $y = \mathcal{T} - \gamma(\mathcal{S})$. 
To train a GP, we can first define the marginal likelihood as
\begin{equation}
    p({y}|{X})= \int p({y}|{f},{X}) p({f}|{X}) d {f} ,
\end{equation}
which represents how likely it is to draw our data given our prior distribution, and where $f$ represents our function values. 
Thus if we can maximize this term, we can maximize the probability of the observed data given our model. 
To perform this maximization we can first calculate the logarithm of the integral above to be
\begin{equation}
    \log (p({y} | {X})) = - {\frac{1}{2} ({y}^\top {K}_y^{-1} {y})} - {\frac{1}{2} \log |{K}_y|} - \frac{n}{2} \log(2\pi) ,
    \label{eq:mll}
\end{equation}
where we use the logarithm to remove the exponential from the Gaussian distribution and obtain a sum, $K_y = K(X, X) + \sigma^2_n I$, and $n$ is the number of observed datapoints. 
Finally an optimizer can be used to find hyperparameters which maximize the marginal log likelihood shown above in \eqref{eq:mll}.
In our specific case, we use a zero-mean prior, and for the kernel a squared exponential kernel: 
\begin{equation}
    k(x_i, x_j) = \sigma_{v}^2 \exp\left(-\frac{1}{2}\left(\frac{(x_{i} - x_{j})^2}{\ell^2}\right)\right) ,
    \label{eq:se_kernel}
\end{equation}
which also shows the kernel hyperparameters that are optimized to fit our GP model, the vertical lengthscale $\sigma_v$ and horizontal lengthscale $\ell$.
We can then train the GP as outlined above using the marginal log-likelihood to obtain a posterior distribution.
Then, to make predictions, we can condition this posterior distribution on our new test inputs $X_*$ to obtain a predictive mean $\mu_{x_{*}}$ as:
\begin{equation}
    {\mu}_{{x}_*}={K}({X}_*,{X})({K}({X},{X})+ \sigma^2_n {I})^{-1} {y},
    \label{eq:pred_mean}
\end{equation}
as well as the predictive uncertainty ${\Sigma}_{{x}_*}$,
\begin{equation}
    {\Sigma}_{{x}_*}={K}({X}_*,{X}_*)-{K}({X}_*,{X})({K}({X},{X})+ \sigma^2_n {I})^{-1} {K}({X},{X}_*) ,
\end{equation}
with ${K}({X}_*,{X})$ being the cross-covariance between the test inputs and the dataset (calculated using our \textit{fitted} kernel, see \eqref{eq:se_kernel}), ${K}({X},{X})$ the covariance matrix, $\sigma_n$ the process noise, $I$ the identity matrix, $y$ the labels, and ${K}({X}_*,{X}_*)$ the self-covariance of the test inputs. 
The predictive mean shown in \eqref{eq:pred_mean} is then what we use as our non-linear transformation $\psi(x)$. 
Having both the linear and non-linear parts of our map $\Phi_{\mathcal{T}}(x)$ for a set of new target keypoints $\tilde{\mathcal{T}}$, we can then use it to transport $\mathcal{X}$ and $\mathcal{R}$ from a demonstration \((\tilde{{\mathcal{S}}}, {\mathcal{X}}, {\mathcal{R}}, {\mathcal{L}})\) using \eqref{eq:transporation}. 
\subsection*{Experimental setup and protocols}

%\textbf{For Mariano}: {\color{red} Add here a detailed description of the experimental setup FOR EACH EXPERIMENT. Be precise about how you executed the tests, provided the demonstrations, and followed the protocols, etc. We should provide enough information for the whole thing to be repeatable (given the code).}
%

% General setup:
% Franka robot, note that since we use impedance control we weigh the soft arm plus camera, this is about 870 g. We also set the TCP, the point we are tracking during demonstrations and executions, to be 28 cm down from the flange of the franka, this corresponds to a point close to the tip of the soft arm and was found empirically to work best. 
%
As outlined above, we use an off-the-shelf Franka robot for the rigid part of our platform.  During demonstrations, the Dynamixel servos are controlled by the user with the buttons on top of the rigid robot. 
Specifically, different buttons on top of the Franka robot can be used to move either of the servos individually in either a clockwise or counter-clockwise direction, and they can also be moved simultaneously in either a clockwise or counter-clockwise direction.

Since we use impedance control to provide demonstrations and execute trajectories, it is essential to weigh the soft arm and camera and input these values into the custom end effector setup of the Desk software for the robot. 
Moreover, our custom end effector setup also moves the center of mass downwards and changes the tool center point (TCP) to a point 28 cm below the flange, which corresponds to a point near the tip of the soft arm. 
For the perception of keypoints, we use the RealSense D405 camera, and we place AprilTags (fiducial markers) on the relevant objects for our designed tasks. 
We use a 3D-printed attachment to connect the camera to the robot, and then calibrate the camera extrinsics using open-source software found on \url{https://github.com/IFL-CAMP/easy_handeye}. This software utilizes standard algorithms from OpenCV to determine the extrinsics given a set of robot poses and detected marker poses in the camera's frame. 
Before providing a demonstration for a skill, the robot then goes to a pre-designated position where the camera can see the entire workspace, and the positions of the detected source keypoints are saved in the robot base frame. 
We can then make the robot compliant by setting all stiffnesses of the impedance controller to zero, and a human can provide the kinesthetic demonstration for the desired skill. 
At the same time, the user can use the buttons on top of the Franka robot to operate the servos of the soft arm. 
The given demonstration, which includes the rigid robot poses and the servo states, is then recorded at 50 Hz. 
% For an execution, the robot first detects the new target keypoints. Transformation is found using the method described above, which is then also applied to the demonstration.
%
At execution time, the robot again goes to a pre-designated position and detects the new target keypoints. 
Our outlined method is used to generalize the relevant skill, which can then be executed using impedance control.
The control is also executed at 50 Hz, and we use a translational stiffness of 1000 N and rotational stiffness of 35 Nm for all axes. 

%\subsection*{Stacking task}
\paragraph*{Stacking task}
First we empirically establish the reachable workspace where the robot will not go into joint limits or self-collide while trying to  grasp. 
This is \textcolor{red}{x} and \textcolor{red}{y}.
For the demonstration, we position the cups far away from the limits of this workspace: the target pickup location of the red cup (approximately) in the center of the right half of this workspace, and the target stacking location (the location of the yellow cylinder) in the center of the left half of the workspace. 
Moreover, the yellow cup is filled with mass so that it weighs 150 g, as otherwise it was too light and fell over too easily. 
Different fiducial markers are placed on the top of these two cylinders so the source keypoints can then be recorded as outlined above. 
The demonstration for this skill is then provided by approaching the red cylinder, grasping it by operating the soft arm to wrap around it, and then stacking it on the yellow cylinder. 
To test this skill, we then performed 20 trials where the positions of the two objects varied. 
We sampled these new positions randomly within the limits of the workspace, but in the first 10, the new red cylinder position was always sampled from the right half and the yellow cylinder position from the left half.
In the following 10 trials, we then switched the objects, with the red cylinder always on the left and the yellow always on the right. 
The goal was to ensure we also tested configurations which were not too similar to the single demonstration. 
To be able to position the objects, in practice, we used the calibrated camera: the desired positions would be sampled in the robot's frame, and we could then use the calibrated camera extrinsics to project these points onto the current image while the robot was at a pre-designated position. 
We could then visually place the objects approximately at the desired positions.
Note that these sampled positions were then only used for manually placing the objects, we then used the camera again to find the new target keypoints before execution.
Out of the 20 trials, 19 were successful, where we define success as stacking the first object on the second without toppling the stack. 
The single failure occurred due to the first cylinder colliding with the second during the stacking. 
See the results section for a visualization of all the tested pairs of positions for the stacking task. 

\paragraph{Non-prehensile manipulation}
This task innvolved the robot moving an object from several initial locations to other target locations through non-prehensile manipulation, that is, without tightly grasping the object (see main text).
Similarly to the previous task, we again empirically establish a workspace where the robot can reach the target object without reaching joint limits or going into self-collision. 
We then place the target object approximately in the center of the left half of this workspace, and the goal in the center of the right half. 
Both the object and goal have fiducial markers so that their positions can be recorded as the source keypoints. 
We use the 7.0 cm diameter red cylinder as the target object, filled with screws to have a total mass of 150~g.
The kinesthetic demonstration is then provided by the human user, who moves the robot while using the buttons on top of the Franka robot to actuate the soft arm. 
This skill is then tested on 15 new configurations, varying both the position of the object and target goal. 
See the Results section for a visualization of all test configur
We sample these new positions from the reachable workspace determined earlier, with the target object remaining always on the left side and the goal always on the right side. 
To position the objects, we again use the camera and its calibrated extrinsics. 
The desired positions are sampled in the robot's reference frame, and these positions are then projected onto the current image so that the objects can be visually moved to the sampled positions. 
We then detect the target keypoints with the camera after the objects have been placed, the transportation algorithm is applied to the demonstration, and the task is executed. 
For this task, in all 15 trials the robot was able to successfully pull the object to the goal position, where we define success as the cylinder fully covering the target fiducial marker, which is similar in width to the cylinder's diameter. 
\paragraph{Dynamic grasping}
% Small description
This task involved grasping an object at a non-zero velocity (see main text).
% workspace part and demonstration
We again first determine workspace bounds where the object will be reachable and the robot will not collide (with itself or the environment) while performing the task.
As a target object to be grasped we again use the red cylinder with diameter of 7.0 cm, and with screws inside it to have a total mass of 150 g.
We then place the object close to the left bound at $y = -0.25$ m and in the middle of the x-direction bounds at approximately $x = 0.45$ m.
The camera is used to record the source keypoints with this position, and then the demonstration is provided by the human user.
The robot is kinesthetically moved while the buttons in the Franka robot are used to actuate the soft arm to quickly grasp the target object in a fluent motion. 
This skill is then tested on 9 new positions of the target object. 
For this task, since there is only one target object to be grasped and no target goal, instead of randomly sampling we used 9 positions in an equally spaced 3 x 3 grid which covers as much of the workspace as possible; see the Results section for a visualization.  
While the movement from the demonstration is already dynamic and without pausing to grasp, we also further sped up the movement by a factor of 1.5. 
In all 9 tested positions, the robot was able to successfully grasp the object, where we define success as the robot grasping the object without dropping it until the end of the trajectory. 
\paragraph{Manipulation through narrow openings}
This task involved grasping different cylindrical objects through a narrow opening (see the main text).
For the demonstration of this skill the walls were placed on the left side of the robot, in a position where reaching through the gap wouldn't make the robot reach joint limits or self-collide. 
We then used the red cylinder with diameter of 7.0 cm, with no extra mass inside it. 
With this task the main goal was to show the generalization capabilities that the soft arm also provides, thus only two positions were tested: one close to the demonstration where the walls were only translated and not rotated, and a second case where the walls were both translated and rotated. 
In the first position of the walls with only translation, apart from testing with the same object from the demonstration, we also tested the same skill with two other objects, a smaller cylinder with diameter of 6.5 cm and a larger cylinder with diameter 7.5 cm. 
In all of these cases the trials were successful, which we define as the robot grasping the object and not dropping it before the end of the trajectory. 
Finally for the new case with the translated and rotated walls, we tested the skill with the same red cylinder from the demonstration, and the robot was also successful.
\section*{Additional Result: Grasping by twisting}
As an alternative way to manipulate objects, we test if the platform is capable of grasping hollow objects by going inside these and twisting, thus tightening against the surface of the object.
As Figure \ref{fig:pick_hollow} shows, such a strategy indeed works. 
\begin{figure}[th!]
    \centering
    \includegraphics[width = 0.7 \textwidth]{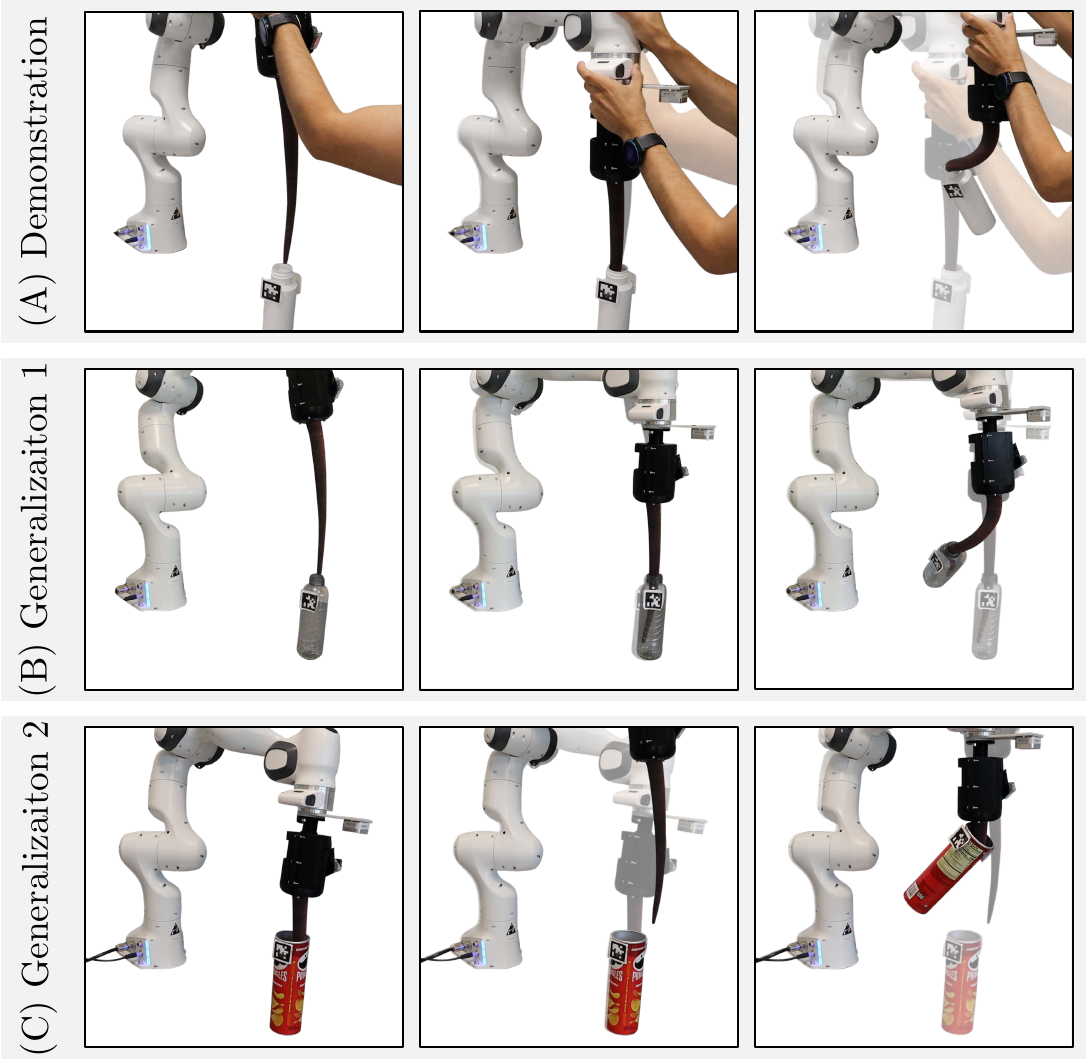}
    \caption{\textbf{Insertion-and-twist task.}  Panel (A) shows the kinesthetic demonstration using a narrow cylindrical object.  Panel (B) depicts execution with a similar albeit different object, while Panel (C) shows generalization to a larger one. Note that in the three examples, the object is located at a different location. No re-training is needed; the soft arm wraps and twists to adapt to the object geometry, enabling successful insertion in both cases.
}
    \label{fig:pick_hollow}
\end{figure}
Moreover, Figure \ref{fig:pick_hollow} shows how such a strategy enables the platform to grab different objects with the same policy: the demonstration is given with the object seen in Figure \ref{fig:pick_hollow}A, but the same policy works for objects of different sizes as shown in Figure \ref{fig:pick_hollow}B and Figure \ref{fig:pick_hollow}C.
\section*{Additional Result: Stacking with three objects}
The platform and generalization are also qualitatively tested on a more difficult stacking task.
In this case an additional larger cylinder has to be stacked on the original target after the first stack, as can be seen in the executions shown in Figure \ref{fig:threestack_task}A and Figure \ref{fig:threestack_task}B.
\begin{figure}
    \centering
    \includegraphics[width=0.8\linewidth]{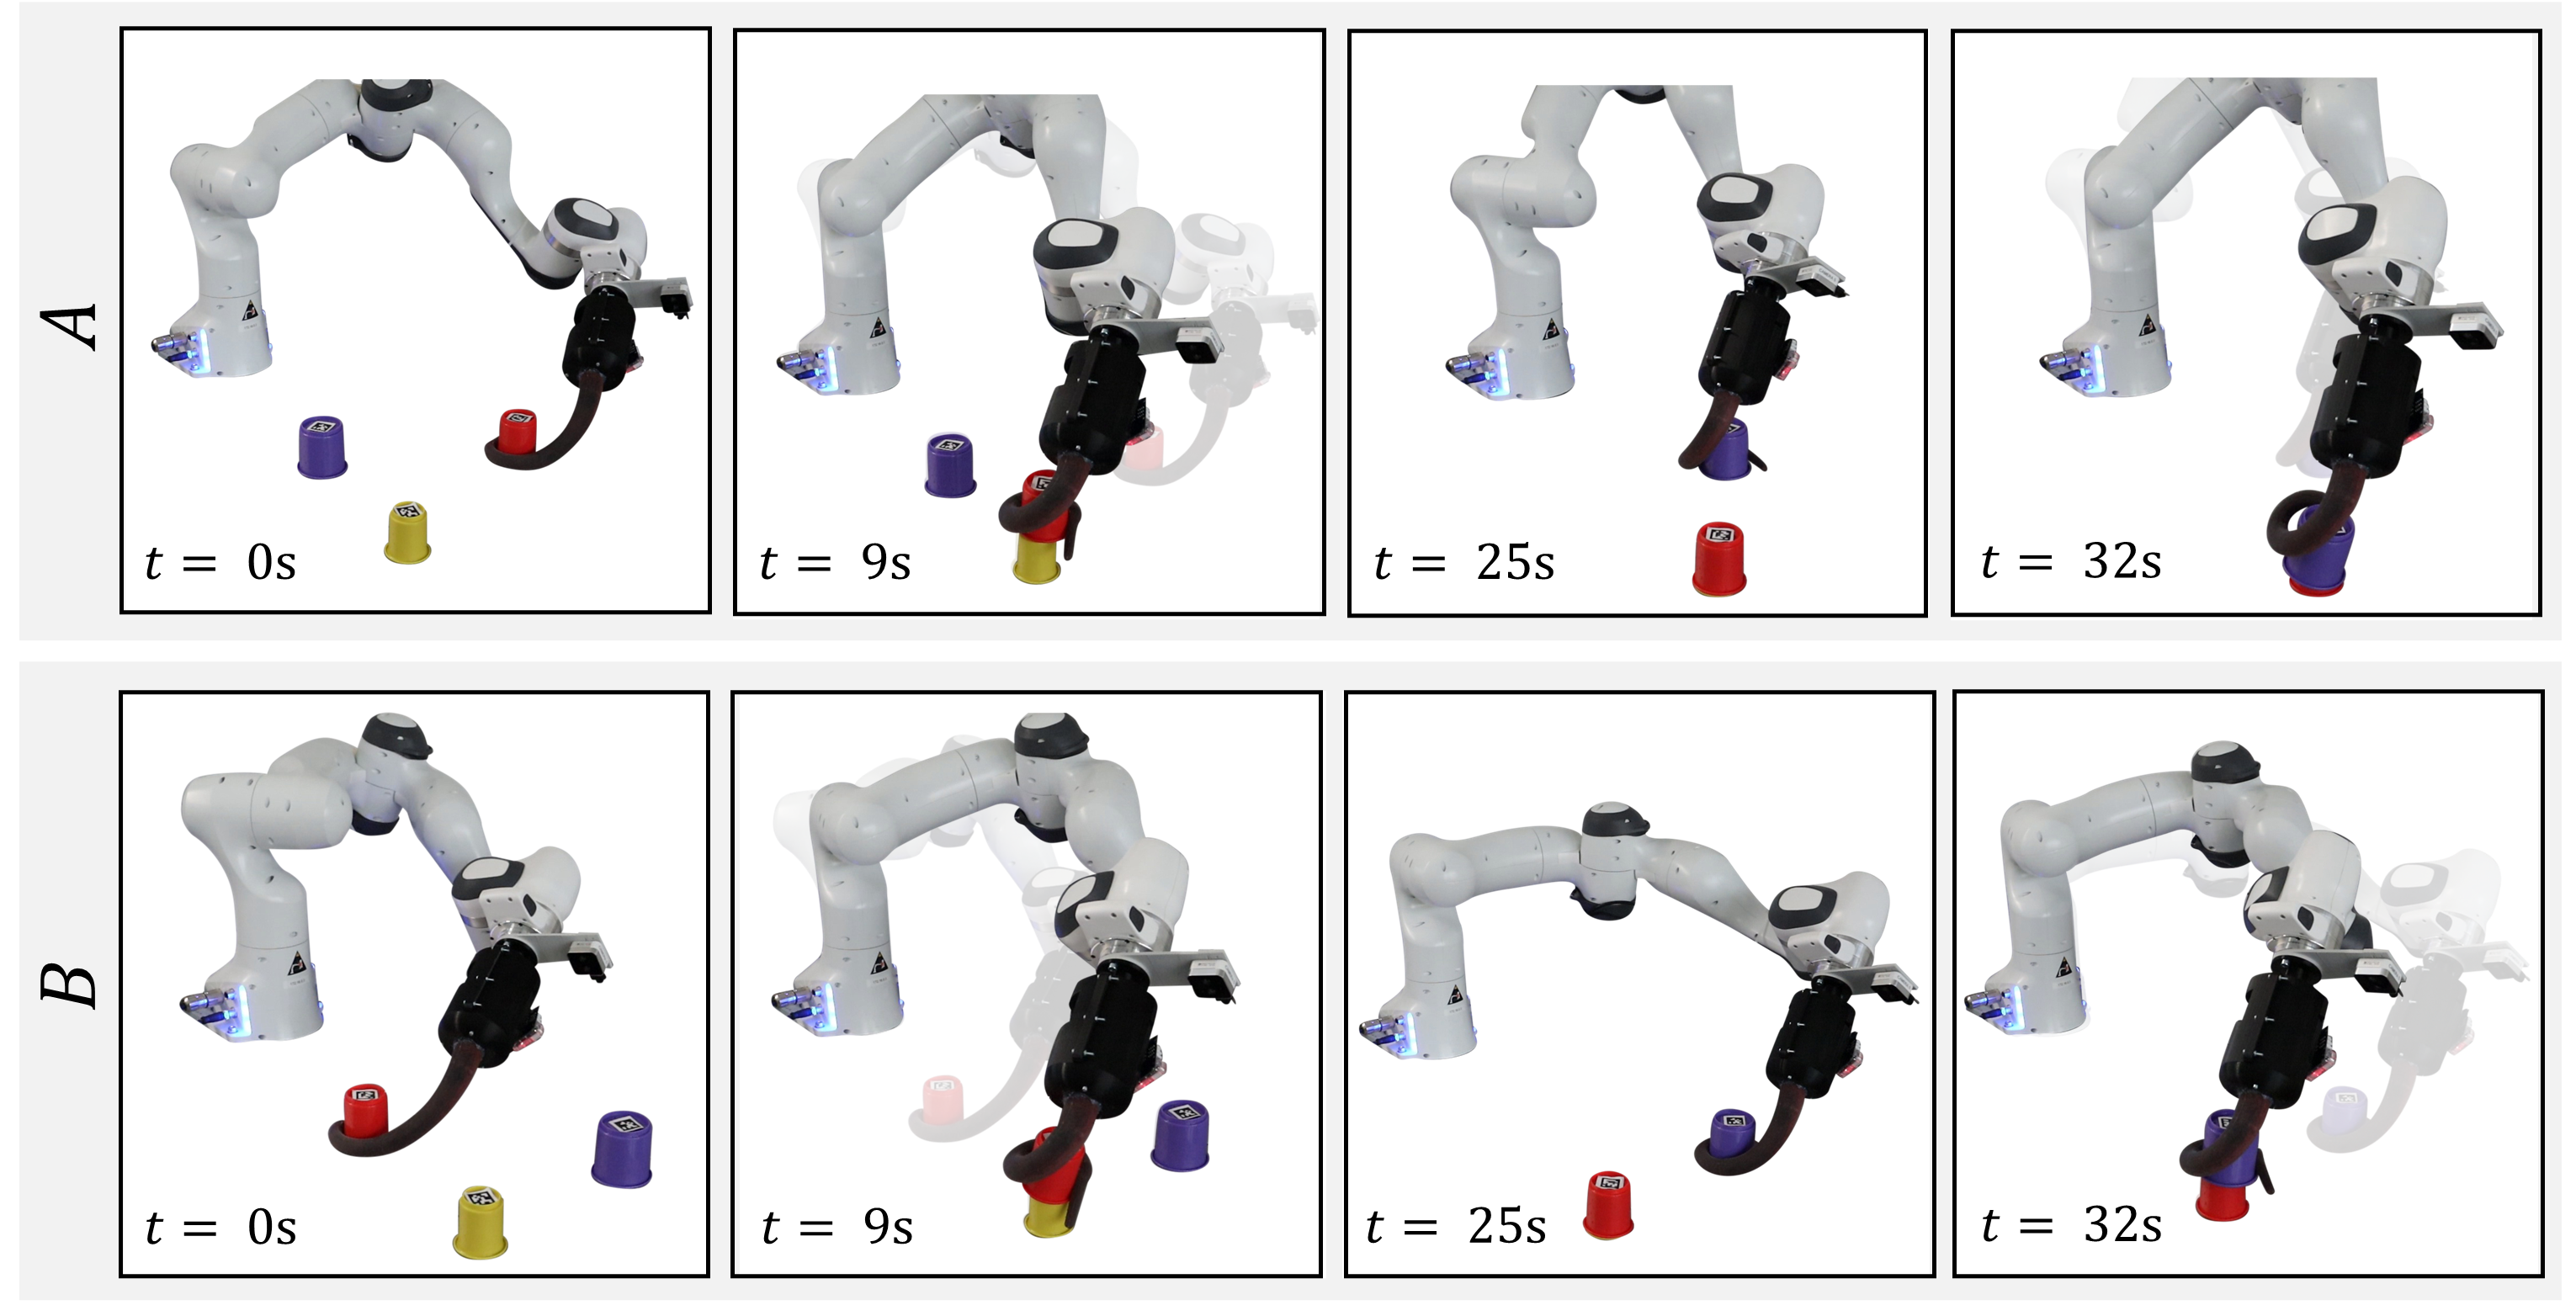}
    \caption{Panel (A) depicts our platform performing a harder stacking task, where two hollow cylinders must be stacked on another target cylinder. Panel (B) then shows an execution where we have swapped the target objects to be picked, a more difficult configuration since it's not as similar to the original demonstration.}
    \label{fig:threestack_task}
\end{figure}
While we did not perform quantitative tests for this task, Figure \ref{fig:threestack_task} shows that is possible to complete this harder task.
Moreover, the second execution shown in Figure \ref{fig:threestack_task}B specifically shows an initial configuration that is different from that of the provided demonstration, where the purple and red cylinders were swapped, similarly to the configuration depicted in Figure \ref{fig:threestack_task}A.
\section*{Additional Result: Characterizations}

\subsection*{Payload characterization}
We are also interested in testing the payload capabilities of our platform. 
Specifically, we aim to investigate how varying object weights and sizes impact the platform's manipulation capabilities. 
We test this through a pick-and-place task, where the object starts at a random location on the left side of the robot and must be moved to a random location on the right side of the robot. 
The task is repeated for different combinations of cylinder weight and diameter to be grasped, and it is repeated 10 times per combination. 
If the full task was completed, a score of 1 was given, if the object was picked but dropped before reaching the goal, a score of 0.5, and finally if the object was not picked up at all, a score of 0 was given. 
We also note that the combination of the smallest diameter cylinder with the largest mass was not possible to test, since the cylinder was completely full before it reached the required weight. 
We can thus get a success rate for this task for each combination, and plot this on a heatmap, as visualized in Figure \ref{fig:heatmap}.
What we would expect is the success rate to decrease with increasing weight, which is indeed shown in Figure \ref{fig:heatmap}.
More interestingly, we can also see that the task becomes harder for both too small or too large objects: if we look at the row for a mass of 225 g, both the 6.5 and 8.0 cm radii cases have lower success rates than the 7.0 and 7.5 cm cases. 
Since we are manipulating the object by wrapping around it, it is likely that for too large objects the contact area decreases, leading to lower friction and a lower payload capacity. 
On the other hand, the soft arm has a limit related to how much it can curl while wrapping, meaning that objects that are too small will have a smaller contact area, and objects that are too small will not even have any contact. 
\begin{figure}[th!]
    \centering
    \includegraphics[width=0.7\linewidth]{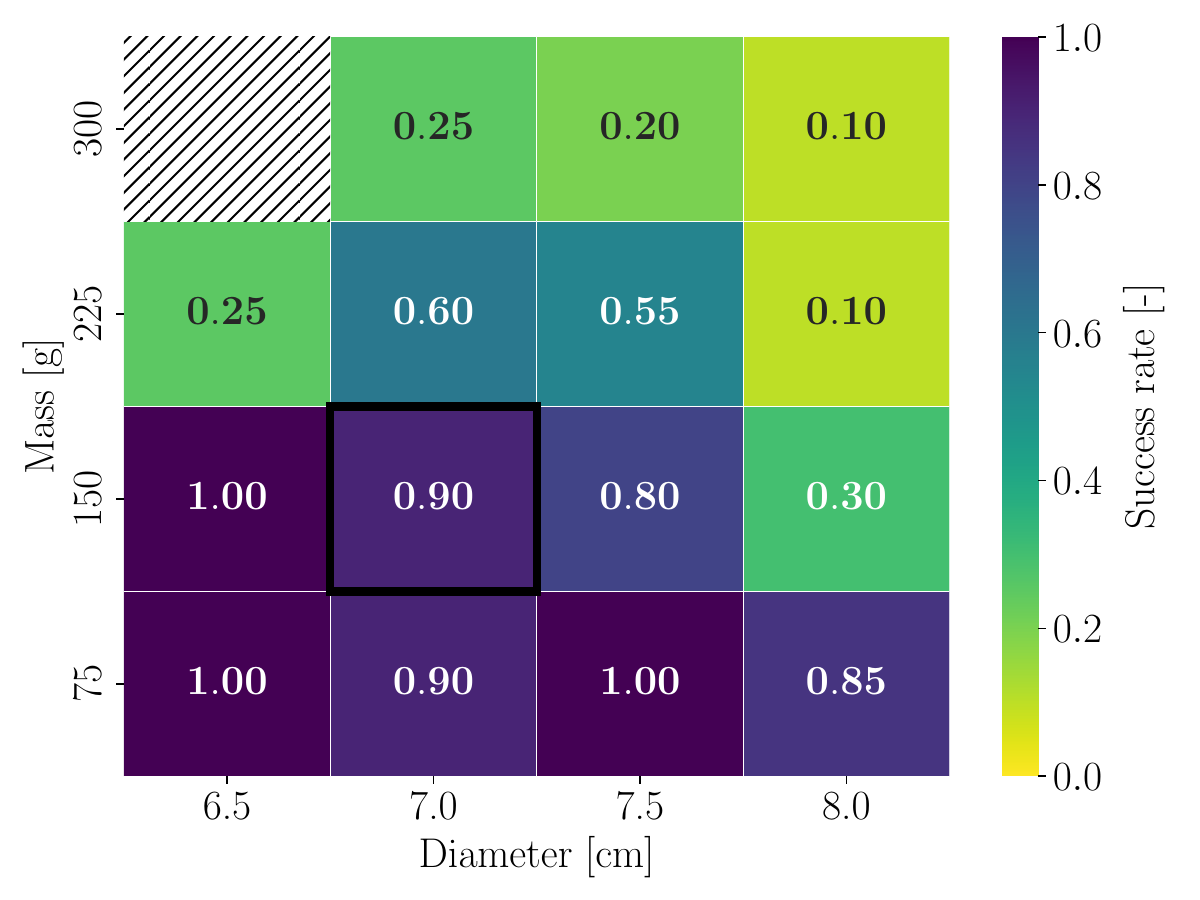}
    \caption{\textbf{Success rates for pick-and-place across object size and weight.}  Heatmap showing success rates over 10 trials for combinations of object diameter and mass. Lighter and smaller objects are handled reliably, while performance degrades as mass and size increase.
}
    \label{fig:heatmap}
\end{figure}
We also show all the tested pick locations in Figure \ref{fig:heatmap_locs}, where color and size indicate mass and diameter, respectively. 
On the right in Figure \ref{fig:heatmap_locs_success} we show the same pick locations, but now use color coding to indicate the trial outcome, green for success, yellow for partial success, and red for failure. 
With these plots can see that the successes and failures have no correlation to physical location, but rather to the size and mass of the object, as the heatmap in Figure \ref{fig:heatmap} also showed.
\begin{figure}[t]
    \centering
    {
    \includegraphics[width=0.46\linewidth, trim=0cm 0cm 2cm 0cm, clip]{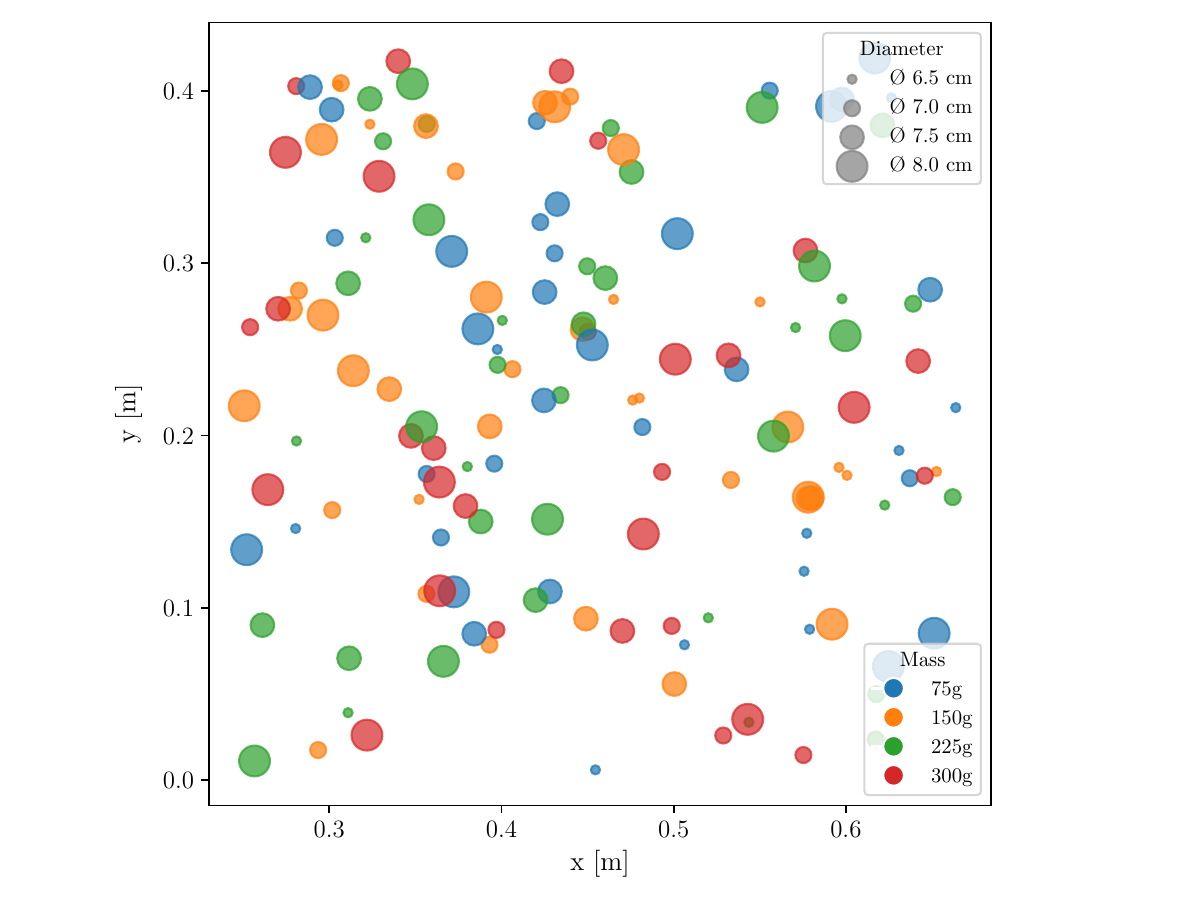}\label{fig:heatmap_locs}}
    \hfill
{
    \includegraphics[width=0.46\linewidth, trim=0cm 0cm 2cm 0cm, clip]{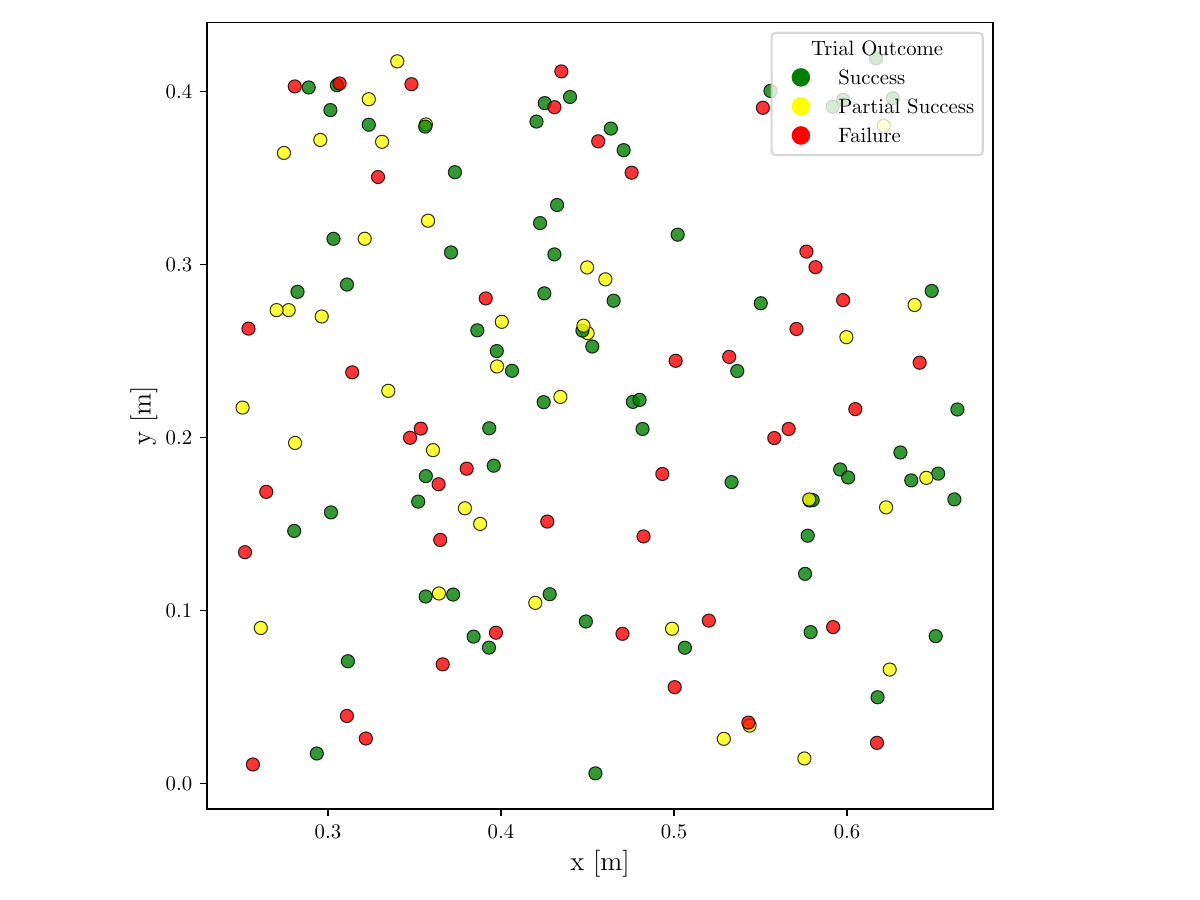}\label{fig:heatmap_locs_success}
    }
    \caption{\textbf{Picking locations during payload capability evaluation.}  The left plot shows picking positions colored by object mass and scaled by object diameter.  The right plot visualizes the outcome of each trial at the corresponding location. The results confirm that success is not correlated with spatial position but depends on object size and weight.}
    \label{fig:heatmap_locs_full}
\end{figure}
\subsection*{Grasping under uncertain perception}
We highlight another advantage of the soft arm by showing how the platform can manipulate objects under uncertain perception situations.
A ``noise" vector of different magnitudes and in different directions (as seen from above, i.e., on the x-y plane) is added to the perceived object location when performing a grasping task. 
We perform this test with magnitudes of 5, 10, and 15 cm for the noise vector, and sample 10 random directions for each of these magnitudes. 
\begin{figure}
    \centering
    \includegraphics[width=0.7\linewidth]{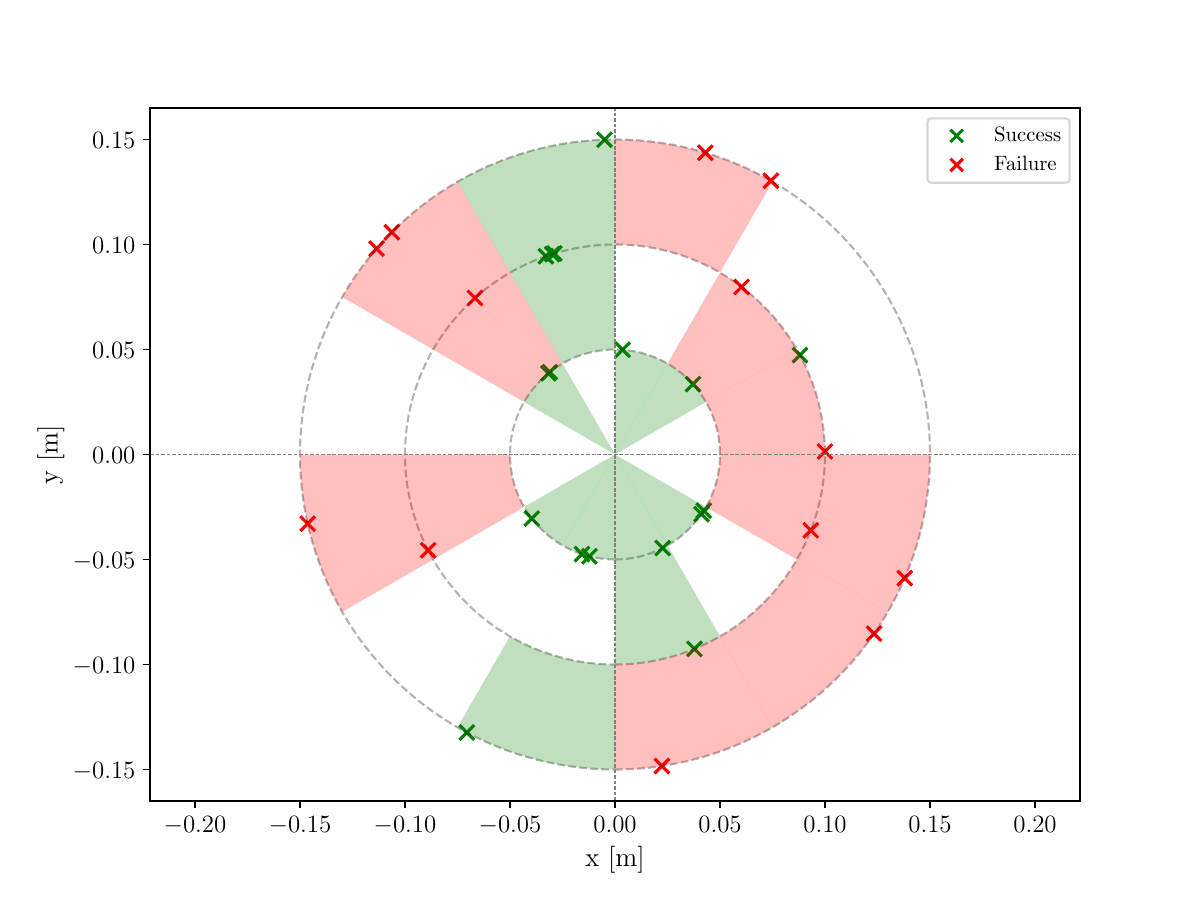}
    \caption{\textbf{Robustness to perception noise in grasping.}  Success and failure regions for perturbed object locations, with the origin representing the true position.  Each point corresponds to a trial with noise added to the perceived target; green areas indicate successful grasps, red areas indicate failures. For comparison, it is worth mentioning that even the inner circle, where the success rate is 100\%, is larger than the maximum size of the standard gripper of the Franka manipulator.}
    \label{fig:noise_plot}
\end{figure}
The results of these tests are shown in Figure \ref{fig:noise_plot}, with the origin representing the real object locations and the markers indicating where the object was perceived after adding the noise, and color indicating success or failure. 
The concentric dashed circles indicate the magnitudes of the noise vectors at 5, 10, or 15 cm.
We then partition the plot into 12 sectors, and further divide these into 36 annular sectors according to the noise magnitude.
If the outer edge of the sector includes a failed grasp, then it is colored red.
If it includes a successful grasp and no failed grasps, then it is colored red.
Sectors without markers but between two green sectors are still considered green, likewise for markerless sectors between two red sectors. 
Finally sectors between a red region and a green region are colored half red and half green.
Green regions thus roughly indicate the range of noise vectors for which the robot can still successfully grasp, and red regions indicate the opposite. 
The first interesting aspect to note from Figure \ref{fig:noise_plot} is that all regions within 5 cm are colored green. 
For reference, a Franka Emika gripper has a maximum open width of 8 cm, meaning that if such a noisy perception then caused a similar error in the position of the end effector, a collision would occur even if the noise vector is aligned with the width-direction of the gripper.
This thus shows an advantage for this ``wrapping" grasping strategy with the soft arm, since the exact position of an object (at least for a similarly sized object as the on in this test) does not need to be so precise. 
Another interesting aspect is the asymmetry for the plot: the robot seems more resistant to noise in the y-direction than in the x-direction. 
However, this is likely due to the specific grasp the test was done with. 
Before starting the wrapping grasp, the soft arm was roughly aligned with the y-axis.
This means that an error in the y-direction would not lead to a collision, and if the object is a bit farther in this direction the wrapping motion can pull the object. 
On the other hand, an error in the negative x-direction would eventually cause a collision, and in the positive direction the soft arm would simply miss the object. 
This plot thus also shows how the specific grasp will naturally influence the success or failure related to specific noise vectors. 
Consequently, in a case where the uncertainty in the perception of the object location is known to be \textit{not} uniform, the grasp strategy could be adjusted to maximize the probablity of success. 

\end{document}
